# Supplementary material for: Diversity Embeddings and the Hypergraph Sparsest Cut
Source: arXiv:2303.04199 source file (2026-11-04)
Supplement: Supplementary file 1 [file appendix.tex]

\chapter{Supporting Materials}

\section{Application of the Triangle Inequality}

\begin{prop}\label{prop:ApplicationOfTriangleIneq}
Let $(X,\delta)$ be a (pseudo) diversity and let $(X,d)$ be its (pseudo) metric space. Let $A=\{v_1,v_2,\ldots,v_k\}\in\mathcal{P}(X)$. Then it follows that

\begin{equation}
    \delta(A) \leq \sum_{i=1}^{k-1}d(v_i,v_{i+1})
\end{equation}
\end{prop}

\begin{proof}
For each $i\in\{1,2,\ldots, k-1\}$ we define
\begin{equation}
    A_i = \{v_1,v_2,\ldots,v_{i+1}\}
\end{equation} Then for any arbitrary $i\in \{2,3,\ldots,k-1\}$ we have that \begin{equation}\label{eqn:appendixeqn1}
    \delta(A_i) \leq \delta(A_{i-1}) + \delta(\{v_i,v_{i+1}\}) = \delta(A_{i-1}) + d(v_i,v_{i+1})
\end{equation} where the inequality follows by the triangle inequality and the fact that $A_{i-1} \cap \{v_i,v_{i+1}\} = \{v_i\} \neq \emptyset$. Then we have that \begin{align}
    \delta(A) & = \delta(A_{k-1}) & \text{by $A_{k-1} = A$} \\
    & \leq \delta(A_{k-2}) + d(v_{k-1},v_k) & \text{by \ref{eqn:appendixeqn1}} \\
    & \leq \delta(A_{k-3}) + d(v_{k-2},v_{k-1}) + d(v_{k-1},v_k) & \text{by \ref{eqn:appendixeqn1}} \\\\
    & \vdots \\
    & \leq \sum_{i=1}^{k-1}d(v_i,v_{i+1}) & \text{by repeated application of \ref{eqn:appendixeqn1}} \\
\end{align} This completes the proof.
\end{proof}

\begin{prop}\label{prop:ApplicationOfTriangleIneq2}
Let $(X,\delta)$ be a (pseudo) diversity and let $(X,d)$ be its (pseudo) metric space. Let $A\in\mathcal{P}(X)$ and $a\in X$ be arbitrary. Then it follows that

\begin{equation}
    \delta(A) \leq \sum_{v\in A}d(v,a)
\end{equation}
\end{prop}

\begin{proof}
First, we enumerate the elements of $A$ as $A= \{v_1,v_2,\ldots,v_k\}$. For each $i\in\{1,2,\ldots, k\}$ we define
\begin{equation}
    A_i = \{a,v_1,v_2,\ldots,v_{i}\}
\end{equation} Then for any arbitrary $i\in \{2,3,\ldots,k\}$ we have that \begin{equation}\label{eqn:appendixeqn2}
    \delta(A_i) \leq \delta(A_{i-1}) + \delta(\{v_i,a\}) = \delta(A_{i-1}) + d(v_i,a)
\end{equation} where the inequality follows by the triangle inequality and the fact that $A_{i-1} \cap \{v_i,a\} = \{a\} \neq \emptyset$. Then we have that \begin{align}
    \delta(A) & \leq \delta(A\cup\{a\}) & \text{by diversities being increasing, Proposition \ref{prop:Monotonicity}} \\
    & = \delta(A_k) & \text{by $A\cup\{a\} = A_k$} \\
    & \leq \delta(A_{k-1}) + d(v_k,a) & \text{by \ref{eqn:appendixeqn2}} \\
    & \leq \delta(A_{k-2}) + d(v_{k-1},a) + d(v_k,a) & \text{by \ref{eqn:appendixeqn2}} \\ 
    & \vdots \\
    & \leq \sum_{v\in A}d(v,a) & \text{by repeated application of \ref{eqn:appendixeqn2}} \\
\end{align} This completes the proof.
\end{proof}
